# Supplementary material for: Redesigning Service Level Agreements: Equity and Efficiency in City Government Operations
Source: arXiv:2410.14825 source file (2026-09-07)
Supplement: Supplementary file 1 [file sup_mat.tex]

% \subsection{Optimization models under other administrative policies}
% \label{subsec:appmodels}

% In this section, we introduce the optimization models generalized for other administrative policies.

\textbf{City budget with borough+category SLAs.}Under this administrative policy, the city maintains a centralized group of inspectors (only one server in the queuing network), and the SLAs are defined for each \{borough, category\} pair (a different queue for incidents of each specification of \{borough, category\}). The optimization problem is as follows, note the absence of the $C_b$ decision variables.
\begin{subequations}
\begin{align}
    &&\min_{\textbf{z}, \phi} \quad  & L(\textbf{z}) = g(\textbf{z}) + f(\textbf{z})\\
    &&\ \text{s.t.}\quad  & -(C\phi_{k,b} - \lambda_{k,b}) z_{k,b} - \alpha \le 0, &&  \forall k\in \mathcal{S}, b\in \mathcal{B},\\
    &&& \sum_{k\in \mathcal{S}, b\in \mathcal{B}} \phi_{k,b} \le 1,  \\
    &&& \phi_{k,b} \ge 0, z_{k,b} \ge 0.
\end{align}
\end{subequations}

% Empirically, we solve the following optimization problem, which enjoys the same properties as outlined by \Cref{prop:opt-reformulation}.
% \begin{subequations}
% \begin{align}
%     \min_{\textbf{x}} \quad  & \tilde L(\textbf{x}) = g(-\alpha\textbf{x}^{-1}) + f(-\alpha\textbf{x}^{-1})\\
%     \ \text{s.t.}\quad  & \sum_{k \in \mathcal{S}, b\in \mathcal{B}} x_{k,b} \le C - \sum_{k\in \mathcal{S}, b\in \mathcal{B}} \lambda_{k,b}\\
%     & x_{k,b} > 0.
% \end{align}
% \end{subequations}

\textbf{City budget with category SLAs.}Under this administrative policy, the city also maintains a centralized group of inspectors, but the SLAs are defined only for each category. The way the SLAs are defined is similar to current practice, where a uniform SLA is imposed on incidents of the same category across the city. The optimization problem is as follows, note the absence of $b$ in the subscripts, indicating that we are not considering borough-specific performance.
\begin{subequations}
\begin{align}
    &&\min_{\textbf{z}, \phi} \quad  & L(\textbf{z}) = g(\textbf{z})\\
    &&\ \text{s.t.}\quad  & -(C\phi_{k} - \lambda_{k}) z_{k} - \alpha \le 0, &&  \forall k\in \mathcal{S},\\
    &&& \sum_{k\in \mathcal{S}} \phi_{k} \le 1,  \\
    &&& \phi_{k} \ge 0, z_{k} \ge 0.
\end{align}
\end{subequations}
